# Supplementary material for: Adversarial Attack Vulnerability of Medical Image Analysis Systems: Unexplored Factors
Source: arXiv:2006.06356 ancillary file (2021-06-17)
Supplement: Supplementary file 1 [file sup_print.pdf]

# Supplementary Material
## Adversarial Attack Vulnerability of Medical Image Analysis Systems: Unexplored Factors

Gerda Bortsova[1,⋆], Cristina González-Gonzalo[2,3,⋆], Suzanne C. Wetstein[4,⋆], Florian Dubost[1], Ioannis Katramados[5], Laurens Hogeweg[5], Bart Liefers[2,3], Bram van Ginneken[6], Josien P.W. Pluim[4], Mitko Veta[4], Clara I. Sánchez[2,3,7], and Marleen de Bruijne[1,8]

[1] Biomedical Imaging Group Rotterdam, Erasmus MC, The Netherlands
[2] A-Eye Research Group, Diagnostic Image Analysis Group, Department of Radiology and Nuclear Medicine, Radboudumc, Nijmegen, The Netherlands
[3] Donders Institute for Brain, Cognition and Behaviour, Radboudumc, Nijmegen, The Netherlands
[4] Medical Image Analysis Group, Department of Biomedical Engineering, Eindhoven University of Technology, Eindhoven, The Netherlands
[5] Intel Corporation, The Netherlands
[6] Diagnostic Image Analysis Group, Department of Radiology and Nuclear Medicine, Radboudumc, Nijmegen, The Netherlands
[7] Department of Ophthalmology. Radboudumc, Nijmegen, The Netherlands
[8] Department of Computer Science, University of Copenhagen, Denmark

⋆ indicates equal contribution

# 1 Perturbation degree

This section includes the results showing the effects of perturbation degree on attack transferability. For each medical application, we include two tables.

The first table shows the **area under the receiver characteristic curve (AUC)** achieved by target models in the test set. This is shown for two model architectures (Inception-v3 and DenseNet-121) and when using FGSM, PGD, or control noise (spatially shuffled black-box adversarial perturbations), with varying perturbation degrees. The target and surrogate models were both randomly initialized and trained with the same dataset, $d1$.

The second table includes the values of the **Structural Similarity Index Measure (SSIM)** between the original images in the test set and the corresponding adversarial images generated with two model architectures (Inception-v3 and DenseNet-121), using FGSM and PGD with varying perturbation degrees.

## 1.1 Ophthalmology

**Table 1.** Effects of perturbation degree on attack transferability. Values show the performance (AUC) of the target models on the images of the test set when adding adversarial noise generated using FGSM, PGD, or control noise (spatially shuffled black-box adversarial perturbations), with varying perturbation degrees. The target and surrogate models were randomly initialized and trained with the same dataset, $d1$. The lowest AUC value (highest attack transferability) is shown in bold.

| Target | Surrogate | Noise | FGSM | | | | | | PGD | | | | | |
|---|---|---|---|---|---|---|---|---|---|---|---|---|---|---|
| | | $\epsilon =$ | 0.01 | 0.02 | 0.03 | 0.04 | 0.05 | 0.06 | 0.01 | 0.02 | 0.03 | 0.04 | 0.05 | 0.06 |
| Inception-v3 | - | None | 0.88 | | | | | | | | | | | |
| Inception-v3 | Inception-v3 | Adversarial | 0.40 | 0.29 | 0.24 | 0.25 | 0.27 | 0.30 | 0.72 | 0.51 | 0.31 | 0.15 | 0.09 | **0.07** |
| Inception-v3 | Inception-v3 | Control | 0.87 | 0.86 | 0.86 | 0.83 | 0.82 | 0.80 | 0.87 | 0.87 | 0.87 | 0.85 | 0.84 | 0.84 |
| Inception-v3 | DenseNet-121 | Adversarial | 0.66 | 0.52 | 0.43 | 0.32 | 0.30 | 0.28 | 0.75 | 0.61 | 0.52 | 0.50 | 0.49 | 0.49 |
| Inception-v3 | DenseNet-121 | Control | 0.87 | 0.87 | 0.86 | 0.83 | 0.81 | 0.80 | 0.87 | 0.87 | 0.87 | 0.87 | 0.87 | 0.87 |
| DenseNet-121 | - | None | 0.84 | | | | | | | | | | | |
| DenseNet-121 | DenseNet-121 | Adversarial | 0.58 | 0.45 | 0.37 | 0.30 | 0.31 | 0.32 | 0.68 | 0.53 | 0.45 | 0.41 | 0.41 | 0.40 |
| DenseNet-121 | DenseNet-121 | Control | 0.84 | 0.83 | 0.82 | 0.76 | 0.71 | 0.66 | 0.84 | 0.83 | 0.83 | 0.82 | 0.82 | 0.82 |
| DenseNet-121 | Inception-v3 | Adversarial | 0.62 | 0.50 | 0.44 | 0.40 | 0.41 | 0.42 | 0.74 | 0.59 | 0.46 | 0.42 | 0.41 | 0.41 |
| DenseNet-121 | Inception-v3 | Control | 0.83 | 0.82 | 0.81 | 0.76 | 0.71 | 0.66 | 0.84 | 0.83 | 0.83 | 0.82 | 0.81 | 0.81 |

**Table 2.** Structural Similarity Index Measure (SSIM) computed between original and adversarial images, generated using FGSM and PGD, with varying perturbation degrees. Values are averaged over all the images in the test set. The highest SSIM value is shown in bold.

| Architecture | FGSM | | | | | | PGD | | | | | |
|---|---|---|---|---|---|---|---|---|---|---|---|---|
| $\epsilon =$ | 0.01 | 0.02 | 0.03 | 0.04 | 0.05 | 0.06 | 0.01 | 0.02 | 0.03 | 0.04 | 0.05 | 0.06 |
| Inception-v3 | 0.97 | 0.92 | 0.85 | 0.71 | 0.64 | 0.58 | **0.98** | 0.94 | 0.90 | 0.85 | 0.82 | 0.82 |
| DenseNet-121 | 0.97 | 0.92 | 0.85 | 0.69 | 0.62 | 0.56 | **0.98** | 0.95 | 0.93 | 0.92 | 0.92 | 0.92 |

## 1.2 Radiology

**Table 3.** Effects of perturbation degree on attack transferability. Values show the performance (AUC) of the target models on the images of the test set when adding adversarial noise generated using FGSM, PGD, or control noise (spatially shuffled black-box adversarial perturbations), with varying perturbation degrees. The target and surrogate models were randomly initialized and trained with the same dataset, $d1$. The lowest AUC value (highest attack transferability) is shown in bold.

| Target | Surrogate | Noise | FGSM | | | | | | PGD | | | | | |
|---|---|---|---|---|---|---|---|---|---|---|---|---|---|---|
| | | $\epsilon =$ | 0.01 | 0.02 | 0.03 | 0.04 | 0.05 | 0.06 | 0.01 | 0.02 | 0.03 | 0.04 | 0.05 | 0.06 |
| Inception-v3 | - | None | 0.75 | | | | | | | | | | | |
| Inception-v3 | Inception-v3 | Adversarial | 0.48 | 0.42 | 0.41 | 0.43 | 0.45 | 0.46 | 0.54 | 0.41 | 0.36 | 0.34 | **0.32** | **0.32** |
| Inception-v3 | Inception-v3 | Control | 0.75 | 0.75 | 0.75 | 0.74 | 0.73 | 0.71 | 0.76 | 0.75 | 0.75 | 0.75 | 0.74 | 0.74 |
| Inception-v3 | DenseNet-121 | Adversarial | 0.66 | 0.6 | 0.56 | 0.55 | 0.55 | 0.55 | 0.69 | 0.61 | 0.56 | 0.52 | 0.5 | 0.48 |
| Inception-v3 | DenseNet-121 | Control | 0.76 | 0.75 | 0.75 | 0.74 | 0.73 | 0.71 | 0.75 | 0.75 | 0.75 | 0.75 | 0.74 | 0.74 |
| DenseNet-121 | - | None | 0.74 | | | | | | | | | | | |
| DenseNet-121 | DenseNet-121 | Adversarial | 0.61 | 0.53 | 0.49 | 0.47 | 0.48 | 0.49 | 0.65 | 0.56 | 0.5 | 0.45 | 0.41 | 0.39 |
| DenseNet-121 | DenseNet-121 | Control | 0.75 | 0.75 | 0.74 | 0.74 | 0.74 | 0.73 | 0.75 | 0.75 | 0.74 | 0.74 | 0.74 | 0.74 |
| DenseNet-121 | Inception-v3 | Adversarial | 0.7 | 0.66 | 0.63 | 0.6 | 0.59 | 0.58 | 0.72 | 0.7 | 0.68 | 0.66 | 0.64 | 0.62 |
| DenseNet-121 | Inception-v3 | Control | 0.75 | 0.75 | 0.74 | 0.74 | 0.73 | 0.73 | 0.75 | 0.75 | 0.75 | 0.74 | 0.74 | 0.74 |

**Table 4.** Structural Similarity Index Measure (SSIM) computed between original and adversarial images, generated using FGSM and PGD, with varying perturbation degrees. Values are averaged over all the images in the test set. The highest SSIM value is shown in bold.

| Architecture | FGSM | | | | | | PGD | | | | | |
|---|---|---|---|---|---|---|---|---|---|---|---|---|
| $\epsilon =$ | 0.01 | 0.02 | 0.03 | 0.04 | 0.05 | 0.06 | 0.01 | 0.02 | 0.03 | 0.04 | 0.05 | 0.06 |
| Inception-v3 | **0.99** | 0.95 | 0.89 | 0.82 | 0.74 | 0.67 | **0.99** | 0.97 | 0.93 | 0.89 | 0.86 | 0.83 |
| DenseNet-121 | **0.99** | 0.95 | 0.89 | 0.83 | 0.75 | 0.69 | **0.99** | 0.96 | 0.93 | 0.89 | 0.86 | 0.83 |

### 1.3 Pathology

**Table 5.** Effects of perturbation degree on attack transferability. Values show the performance (AUC) of the target models on the images of the test set when adding adversarial noise generated using FGSM, PGD, or control noise (spatially shuffled black-box adversarial perturbations), with varying perturbation degrees. The target and surrogate models were randomly initialized and trained with the same dataset, $d1$. The lowest AUC value (highest attack transferability) is shown in bold.

| Target | Surrogate | Noise | FGSM | | | | | | PGD | | | | | |
|---|---|---|---|---|---|---|---|---|---|---|---|---|---|---|
| | | $\epsilon =$ | 0.01 | 0.02 | 0.03 | 0.04 | 0.05 | 0.06 | 0.01 | 0.02 | 0.03 | 0.04 | 0.05 | 0.06 |
| Inception-v3 | - | None | 0.86 | | | | | | | | | | | |
| Inception-v3 | Inception-v3 | Adversarial | 0.66 | 0.47 | 0.34 | 0.27 | 0.24 | 0.24 | 0.67 | 0.44 | 0.30 | 0.22 | 0.18 | 0.16 |
| Inception-v3 | Inception-v3 | Control | 0.84 | 0.84 | 0.84 | 0.84 | 0.84 | 0.84 | 0.84 | 0.84 | 0.84 | 0.84 | 0.84 | 0.84 |
| Inception-v3 | DenseNet-121 | Adversarial | 0.78 | 0.72 | 0.67 | 0.64 | 0.62 | 0.60 | 0.78 | 0.75 | 0.75 | 0.75 | 0.75 | 0.75 |
| Inception-v3 | DenseNet-121 | Control | 0.84 | 0.84 | 0.84 | 0.84 | 0.84 | 0.84 | 0.84 | 0.84 | 0.84 | 0.84 | 0.84 | 0.84 |
| DenseNet-121 | - | None | 0.87 | | | | | | | | | | | |
| DenseNet-121 | DenseNet-121 | Adversarial | 0.57 | 0.37 | 0.24 | 0.18 | 0.17 | 0.16 | 0.64 | 0.34 | 0.20 | 0.11 | 0.08 | **0.06** |
| DenseNet-121 | DenseNet-121 | Control | 0.89 | 0.89 | 0.89 | 0.89 | 0.89 | 0.89 | 0.89 | 0.89 | 0.89 | 0.89 | 0.89 | 0.89 |
| DenseNet-121 | Inception-v3 | Adversarial | 0.79 | 0.66 | 0.54 | 0.44 | 0.37 | 0.32 | 0.81 | 0.71 | 0.64 | 0.56 | 0.51 | 0.48 |
| DenseNet-121 | Inception-v3 | Control | 0.89 | 0.89 | 0.89 | 0.89 | 0.89 | 0.89 | 0.89 | 0.89 | 0.89 | 0.89 | 0.89 | 0.89 |

**Table 6.** Structural Similarity Index Measure (SSIM) computed between original and adversarial images, generated using FGSM and PGD, with varying perturbation degrees. Values are averaged over all the images in the test set. The highest SSIM value is shown in bold.

| Architecture | FGSM | | | | | | PGD | | | | | |
|---|---|---|---|---|---|---|---|---|---|---|---|---|
| $\epsilon =$ | 0.01 | 0.02 | 0.03 | 0.04 | 0.05 | 0.06 | 0.01 | 0.02 | 0.03 | 0.04 | 0.05 | 0.06 |
| Inception-v3 | **1.00** | 0.99 | 0.98 | 0.97 | 0.96 | 0.94 | **1.00** | 0.99 | 0.99 | 0.98 | 0.98 | 0.98 |
| DenseNet-121 | **1.00** | 0.99 | 0.99 | 0.98 | 0.97 | 0.96 | **1.00** | **1.00** | 0.99 | 0.99 | 0.98 | 0.98 |

## 2 Pre-training on ImageNet

This section focuses on the effects of pre-training and the interaction between pre-training and model architecture parity on attack transferability. For each medical application, the table shows the **area under the receiver characteristic curve (AUC)** achieved by target models for FGSM and PGD ($\epsilon = 0.02$) black-box attacks and two randomly initialized model architectures (Inception-v3 and DenseNet-121). The target and surrogate model were both trained with the same dataset, $d1$. Relative performance with respect to the no-attack setting is shown in brackets.

### 2.1 Ophthalmology

**Table 7.** Effects of pre-training on attack transferability. Values show the performance (AUC) of the target models on the images of the test set adversarially perturbed using FGSM or PGD. The target and surrogate model were both trained with the same dataset, $d1$. Relative performance with respect to the no-attack setting is shown in brackets. The lowest AUC value (highest attack transferability) is shown in bold.

| Target | Surrogate | FGSM | PGD |
|---|---|---|---|
| Inception-v3 - ImageNet | - | 0.95 | |
| Inception-v3 - ImageNet | Inception-v3 - ImageNet | **0.00 (0%)** | **0.00 (0%)** |
| Inception-v3 - ImageNet | Inception-v3 - Random | 0.69 (72%) | 0.72 (75%) |
| Inception-v3 - ImageNet | DenseNet-121 - Imagenet | 0.32 (33%) | 0.28 (29%) |
| Inception-v3 - ImageNet | DenseNet-121- Random | 0.86 (90%) | 0.89 (93%) |
| Inception-v3 - Random | - | 0.88 | |
| Inception-v3 - Random | Inception-v3 - ImageNet | 0.52 (59%) | 0.50 (56%) |
| Inception-v3 - Random | Inception-v3 - Random | 0.29 (32%) | 0.51 (57%) |
| Inception-v3 - Random | DenseNet-121 - Imagenet | 0.69 (79%) | 0.75 (84%) |
| Inception-v3 - Random | DenseNet-121- Random | 0.52 (59%) | 0.61 (69%) |
| DenseNet-121 - ImageNet | - | 0.93 | |
| DenseNet-121 - ImageNet | Inception-v3 - ImageNet | 0.20 (21%) | 0.16 (17%) |
| DenseNet-121 - ImageNet | Inception-v3 - Random | 0.83 (88%) | 0.86 (92%) |
| DenseNet-121 - ImageNet | DenseNet-121 - Imagenet | 0.01 (1%) | **0.00 (0%)** |
| DenseNet-121 - ImageNet | DenseNet-121- Random | 0.88 (93%) | 0.90 (96%) |
| DenseNet-121 - Random | - | 0.84 | |
| DenseNet-121 - Random | Inception-v3 - ImageNet | 0.69 (82%) | 0.72 (85%) |
| DenseNet-121 - Random | Inception-v3 - Random | 0.50 (59%) | 0.59 (69%) |
| DenseNet-121 - Random | DenseNet-121 - Imagenet | 0.74 (88%) | 0.78 (92%) |
| DenseNet-121 - Random | DenseNet-121 - Random | 0.45 (53%) | 0.53 (62%) |

### 2.2 Radiology

**Table 8.** Effects of pre-training on attack transferability. Values show the performance (AUC) of the target models on the images of the test set adversarially perturbed using FGSM or PGD. The target and surrogate model were both trained with the same dataset, $d1$. Relative performance with respect to the no-attack setting is shown in brackets. The lowest AUC value (highest attack transferability) is shown in bold.

| Target | Surrogate | FGSM | PGD |
|---|---|---|---|
| Inception-v3 - ImageNet | - | 0.77 | |
| Inception-v3 - ImageNet | Inception-v3 - ImageNet | 0.31 (40%) | 0.34 (44%) |
| Inception-v3 - ImageNet | Inception-v3 - Random | 0.46 (60%) | 0.49 (64%) |
| Inception-v3 - ImageNet | DenseNet-121 - ImageNet | 0.47 (60%) | 0.51 (66%) |
| Inception-v3 - ImageNet | DenseNet-121 - Random | 0.61 (79%) | 0.63 (81%) |
| Inception-v3 - Random | - | 0.76 | |
| Inception-v3 - Random | Inception-v3 - ImageNet | 0.53 (71%) | 0.58 (77%) |
| Inception-v3 - Random | Inception-v3 - Random | 0.42 (55%) | 0.41 (54%) |
| Inception-v3 - Random | DenseNet-121 - ImageNet | 0.57 (75%) | 0.62 (82%) |
| Inception-v3 - Random | DenseNet-121 - Random | 0.60 (79%) | 0.61 (80%) |
| DenseNet-121 - ImageNet | - | 0.78 | |
| DenseNet-121 - ImageNet | Inception-v3 - ImageNet | 0.48 (62%) | 0.56 (72%) |
| DenseNet-121 - ImageNet | Inception-v3 - Random | 0.53 (68%) | 0.58 (74%) |
| DenseNet-121 - ImageNet | DenseNet-121 - ImageNet | **0.28 (36%)** | 0.30 (38%) |
| DenseNet-121 - ImageNet | DenseNet-121 - Random | 0.62 (80%) | 0.63 (81%) |
| DenseNet-121 - Random | - | 0.75 | |
| DenseNet-121 - Random | Inception-v3 - ImageNet | 0.69 (92%) | 0.72 (96%) |
| DenseNet-121 - Random | Inception-v3 - Random | 0.66 (88%) | 0.70 (94%) |
| DenseNet-121 - Random | DenseNet-121 - ImageNet | 0.8 (91%) | 0.71 (95%) |
| DenseNet-121 - Random | DenseNet-121 - Random | 0.53 (71%) | 0.56 (75%) |

### 2.3 Pathology

**Table 9.** Effects of pre-training on attack transferability. Values show the performance (AUC) of the target models on the images of the test set adversarially perturbed using FGSM or PGD. The target and surrogate model were both trained with the same dataset, $d1$. Relative performance with respect to the no-attack setting is shown in brackets. The lowest AUC value (highest attack transferability) is shown in bold.

| Target | Surrogate | FGSM | PGD |
|---|---|---|---|
| Inception-v3 - ImageNet | - | 0.85 | |
| Inception-v3 - ImageNet | Inception-v3 - ImageNet | 0.67 (79%) | 0.72 (85%) |
| Inception-v3 - ImageNet | Inception-v3 - Random | 0.67 (79%) | 0.71 (84%) |
| Inception-v3 - ImageNet | DenseNet-121 - Imagenet | 0.78 (92%) | 0.80 (94%) |
| Inception-v3 - ImageNet | DenseNet-121- Random | 0.78 (92%) | 0.80 (94%) |
| Inception-v3 - Random | - | 0.84 | |
| Inception-v3 - Random | Inception-v3 - ImageNet | 0.50 (60%) | 0.49 (58%) |
| Inception-v3 - Random | Inception-v3 - Random | 0.47 (56%) | 0.44 (52%) |
| Inception-v3 - Random | DenseNet-121 - Imagenet | 0.71 (85%) | 0.74 (88%) |
| Inception-v3 - Random | DenseNet-121- Random | 0.72 (86%) | 0.75 (89%) |
| DenseNet-121 - ImageNet | - | 0.89 | |
| DenseNet-121 - ImageNet | Inception-v3 - ImageNet | 0.71 (80%) | 0.71 (80%) |
| DenseNet-121 - ImageNet | Inception-v3 - Random | 0.68 (76%) | 0.73 (82%) |
| DenseNet-121 - ImageNet | DenseNet-121 - Imagenet | 0.50 (56%) | 0.54 (61%) |
| DenseNet-121 - ImageNet | DenseNet-121- Random | 0.71 (80%) | 0.76 (85%) |
| DenseNet-121 - Random | - | 0.89 | |
| DenseNet-121 - Random | Inception-v3 - ImageNet | 0.66 (74%) | 0.66 (74%) |
| DenseNet-121 - Random | Inception-v3 - Random | 0.66 (74%) | 0.71 (80%) |
| DenseNet-121 - Random | DenseNet-121 - Imagenet | 0.69 (78%) | 0.73 (82%) |
| DenseNet-121 - Random | DenseNet-121 - Random | 0.37 (42%) | **0.34 (38%)** |

## 3 Development data disparity

This section focuses on the effects of data and model architecture parity on attack transferability. The performance (**area under the receiver characteristic curve (AUC)**) of FGSM and PGD ($\epsilon = 0.02$) black-box attacks and two randomly initialized model architectures (Inception-v3 and DenseNet-121) is shown. Target models are trained on $d1$, while surrogate models are trained on different development sets.

### 3.1 Ophthalmology

**Table 10.** Effects of data parity on attack transferability. Performance (AUC) at $\epsilon = 0.02$ is shown, with surrogate models trained on different sets while the target model is trained on $d1$. Relative performance with respect to the no-attack setting is shown in brackets. The lowest AUC value (highest attack transferability) is shown in bold.

| Target | Surrogate | Training set | FGSM | PGD |
|---|---|---|---|---|
| Inception-v3 | - | - | 0.88 | |
| Inception-v3 | Inception-v3 | d1 | **0.29 (32%)** | 0.51 (57%) |
| Inception-v3 | Inception-v3 | d2 | 0.54 (62%) | 0.74 (83%) |
| Inception-v3 | Inception-v3 | d2/2 | 0.72 (81%) | 0.77 (87%) |
| Inception-v3 | DenseNet-121 | d1 | 0.52 (59%) | 0.61 (69%) |
| Inception-v3 | DenseNet-121 | d2 | 0.58 (65%) | 0.62 (70%) |
| Inception-v3 | DenseNet-121 | d2/2 | 0.84 (96%) | 0.85 (97%) |
| DenseNet-121 | - | - | 0.84 | |
| DenseNet-121 | DenseNet-121 | d1 | 0.45 (53%) | 0.53 (62%) |
| DenseNet-121 | DenseNet-121 | d2 | 0.45 (53%) | 0.51 (60%) |
| DenseNet-121 | DenseNet-121 | d2/2 | 0.76 (90%) | 0.76 (90%) |
| DenseNet-121 | Inception-v3 | d1 | 0.50 (59%) | 0.59 (69%) |
| DenseNet-121 | Inception-v3 | d2 | 0.66 (78%) | 0.78 (92%) |
| DenseNet-121 | Inception-v3 | d2/2 | 0.73 (86%) | 0.77 (91%) |

**Table 11.** Transferability of attacks on models trained on small datasets in a data disparity scenario. Performance (AUC) at $\epsilon = 0.02$ is shown, with surrogate models trained on $d2$ while the target model is trained on $d1/10$. Relative performance with respect to the no-attack setting is shown in brackets. The lowest AUC value (highest attack transferability) is shown in bold.

| Target | Surrogate | FGSM | PGD |
|---|---|---|---|
| Inception-v3 - ImageNet | - | 0.88 | |
| Inception-v3 - ImageNet | Inception-v3 - ImageNet | 0.27 (31%) | 0.08 (9%) |
| Inception-v3 - ImageNet | DenseNet-121 - ImageNet | 0.37 (42%) | 0.22 (24%) |
| Inception-v3 - Random | - | 0.63 | |
| Inception-v3 - Random | Inception-v3 - Random | 0.62 (98%) | 0.62 (98%) |
| Inception-v3 - Random | DenseNet-121- Random | 0.62 (98%) | 0.62 (98%) |
| DenseNet-121 - ImageNet | - | 0.87 | |
| DenseNet-121 - ImageNet | Inception-v3 - ImageNet | 0.59 (67%) | 0.60 (69%) |
| DenseNet-121 - ImageNet | DenseNet-121 - ImageNet | 0.16 (18%) | **0.01 (1%)** |
| DenseNet-121 - Random | - | 0.58 | |
| DenseNet-121 - Random | Inception-v3 - Random | 0.58 (100%) | 0.58 (100%) |
| DenseNet-121 - Random | DenseNet-121 - Random | 0.58 (100%) | 0.58 (100%) |

### 3.2 Radiology

**Table 12.** Effects of data parity on attack transferability. Performance (AUC) at $\epsilon = 0.02$ is shown, with surrogate models trained on different sets while the target model is trained on $d1$. Relative performance with respect to the no-attack setting is shown in brackets. The lowest AUC value (highest attack transferability) is shown in bold.

| Target | Surrogate | Training set | FGSM | PGD |
|---|---|---|---|---|
| Inception-v3 | - | - | 0.75 | |
| Inception-v3 | Inception-v3 | d1 | 0.42 (55%) | **0.41 (54%)** |
| Inception-v3 | Inception-v3 | d2 | 0.52 (68%) | 0.54 (71%) |
| Inception-v3 | Inception-v3 | d2/2 | 0.60 (79%) | 0.59 (78%) |
| Inception-v3 | DenseNet-121 | d1 | 0.60 (79%) | 0.61 (80%) |
| Inception-v3 | DenseNet-121 | d2 | 0.62 (82%) | 0.62 (82%) |
| Inception-v3 | DenseNet-121 | d2/2 | 0.67 (89%) | 0.67 (89%) |
| DenseNet-121 | - | - | 0.74 | |
| DenseNet-121 | DenseNet-121 | d1 | 0.53 (71%) | 0.56 (75%) |
| DenseNet-121 | DenseNet-121 | d2 | 0.59 (79%) | 0.62 (83%) |
| DenseNet-121 | DenseNet-121 | d2/2 | 0.59 (79%) | 0.59 (80%) |
| DenseNet-121 | Inception-v3 | d1 | 0.66 (88%) | 0.70 (94%) |
| DenseNet-121 | Inception-v3 | d2 | 0.66 (88%) | 0.70 (94%) |
| DenseNet-121 | Inception-v3 | d2/2 | 0.69 (93%) | 0.71 (95%) |

**Table 13.** Transferability of attacks on models trained on small datasets in a data disparity scenario. Performance (AUC) at $\epsilon = 0.02$ is shown, with surrogate models trained on $d2$ while the target model is trained on $d1/10$. Relative performance with respect to the no-attack setting is shown in brackets. The lowest AUC value (highest attack transferability) is shown in bold.

| Target | Surrogate | FGSM | PGD |
|---|---|---|---|
| Inception-v3 - ImageNet | - | 0.68 | |
| Inception-v3 - ImageNet | Inception-v3 - ImageNet | **0.53 (78%)** | 0.56 (82%) |
| Inception-v3 - ImageNet | DenseNet-121 - ImageNet | 0.62 (91%) | 0.63 (93%) |
| Inception-v3 - Random | - | 0.64 | |
| Inception-v3 - Random | Inception-v3 - Random | 0.63 (99%) | 0.63 (99%) |
| Inception-v3 - Random | DenseNet-121- Random | 0.63 (99%) | 0.64 (99%) |
| DenseNet-121 - ImageNet | - | 0.69 | |
| DenseNet-121 - ImageNet | Inception-v3 - ImageNet | 0.59 (85%) | 0.63 (91%) |
| DenseNet-121 - ImageNet | DenseNet-121 - ImageNet | 0.61 (89%) | 0.62 (89%) |
| DenseNet-121 - Random | - | 0.63 | |
| DenseNet-121 - Random | Inception-v3 - Random | 0.63 (99%) | 0.63 (100%) |
| DenseNet-121 - Random | DenseNet-121 - Random | 0.63 (99%) | 0.63 (100%) |

### 3.3 Pathology

**Table 14.** Effects of data parity on attack transferability. Performance (AUC) at $\epsilon = 0.02$ is shown, with surrogate models trained on different sets while the target model is trained on $d1$. Relative performance with respect to the no-attack setting is shown in brackets. The lowest AUC value (highest attack transferability) is shown in bold.

| Target | Surrogate | Training set | FGSM | PGD |
|---|---|---|---|---|
| Inception-v3 | - | - | 0.84 | |
| Inception-v3 | Inception-v3 | d1 | 0.47 (56%) | 0.44 (52%) |
| Inception-v3 | Inception-v3 | d2 | 0.62 (74%) | 0.66 (79%) |
| Inception-v3 | Inception-v3 | d2/2 | 0.62 (74%) | 0.66 (79%) |
| Inception-v3 | DenseNet-121 | d1 | 0.72 (86%) | 0.75 (89%) |
| Inception-v3 | DenseNet-121 | d2 | 0.70 (83%) | 0.71 (85%) |
| Inception-v3 | DenseNet-121 | d2/2 | 0.64 (76%) | 0.65 (77%) |
| DenseNet-121 | - | - | 0.89 | |
| DenseNet-121 | DenseNet-121 | d1 | 0.37 (42%) | **0.34 (38%)** |
| DenseNet-121 | DenseNet-121 | d2 | 0.69 (78%) | 0.70 (79%) |
| DenseNet-121 | DenseNet-121 | d2/2 | 0.65 (73%) | 0.65 (73%) |
| DenseNet-121 | Inception-v3 | d1 | 0.66 (74%) | 0.71 (80%) |
| DenseNet-121 | Inception-v3 | d2 | 0.75 (84%) | 0.78 (88%) |
| DenseNet-121 | Inception-v3 | d2/2 | 0.75 (84%) | 0.78 (88%) |

**Table 15.** Transferability of attacks on models trained on small datasets in a data disparity scenario. Performance (AUC) at $\epsilon = 0.02$ is shown, with surrogate models trained on $d2$ while the target model is trained on $d1/10$. Relative performance with respect to the no-attack setting is shown in brackets. The lowest AUC value (highest attack transferability) is shown in bold.

| Target | Surrogate | FGSM | PGD |
|---|---|---|---|
| Inception-v3 - ImageNet | - | 0.73 | |
| Inception-v3 - ImageNet | Inception-v3 - ImageNet | **0.66 (90%)** | 0.67 (92%) |
| Inception-v3 - ImageNet | DenseNet-121 - ImageNet | 0.71 (97%) | 0.72 (99%) |
| Inception-v3 - Random | - | 0.79 | |
| Inception-v3 - Random | Inception-v3 - Random | 0.78 (99%) | 0.78 (99%) |
| Inception-v3 - Random | DenseNet-121- Random | 0.79 (100%) | 0.79 (100%) |
| DenseNet-121 - ImageNet | - | 0.83 | |
| DenseNet-121 - ImageNet | Inception-v3 - ImageNet | 0.80 (96%) | 0.80 (96%) |
| DenseNet-121 - ImageNet | DenseNet-121 - ImageNet | 0.77 (93%) | 0.77 (93%) |
| DenseNet-121 - Random | - | 0.84 | |
| DenseNet-121 - Random | Inception-v3 - Random | 0.79 (94%) | 0.79 (94%) |
| DenseNet-121 - Random | DenseNet-121 - Random | 0.79 (94%) | 0.81 (96%) |
